# Supplementary material for: Supersymmetry and the Spectral Action. On a geometrical interpretation of the MSSM
Source: arXiv:1409.6751 source file (2014-09-23)
Supplement: Supplementary file 1 [file Superfields.tex]

\section{The superfield formalism}\label{sec:superfields}
